# Supplementary material for: Cinematic-L1 Video Stabilization with a Log-Homography Model
Source: arXiv:2011.08144 ancillary file (2020-11-20)
Supplement: Supplementary file 1 [file l1_stabilization_supplement.pdf]

# Supplementary Material for Cinematic-L1 Video Stabilization with a Log-Homography Model

Arwen Bradley, Jason Klivington, Joseph Triscari, Rudolph van der Merwe  
Apple, Inc.

{arwen.bradley, klivington, jtriscari, vandermerwe}@apple.com

## A. Results

### A.1. Quantitative comparisons

We follow the quantitative evaluation strategy proposed by [15], comparing our method to five representative stabilization methods: the spatially and temporally optimized method (STO) [12], the bundled camera paths method (BCP) [9], the homography version of geodesic video stabilization (PG2) [15], and two commercial softwares: Adobe After Effect (AE) warp stabilizer (whose algorithm is based on subspace video stabilization [7]), and YouTube stabilizer (based on [2]) (versions as of 2017, when [15] was published). Since our method allows the client to specify the crop budget (which trades-off stabilization strength with amount of crop), we run our method with crop budgets of 10%, 20%, and 30%.

We compare the four criteria proposed by [15]: *running time*, *stability*, *distortion*, and *cropping ratio*. These are described in full detail in [15] but we summarize here. For *running time*, we consider both the total time per frame as well as the time for smoothing/warping only (since the time for analysis of the input motion can be very implementation-dependent and does not necessarily reflect on the speed of the stabilization algorithm itself). *Stability* is admittedly rather subjective, but [15] formulate it in terms of the acceleration of the translation and rotation components of the stabilized motion. *Distortion* is given by the geometric deviation of the two eigenvalues of the affine part of the correction homography matrix. *Cropping ratio* is defined as the ratio of the areas of the stabilized and unstabilized frame. We run the experiments on a public dataset published in [9], consisting of 174 videos divided into categories *simple*, *quick rotation*, *zooming*, *parallax*, *crowd*, *running*.

Results are shown in figure 11 in the main text. Since L1 respects a client-specified crop budget, the *cropping* metric for L1 with a given crop budget is approximately constant for all input videos. (Note that we define the crop fraction in terms of side length while [15]’s *cropping* metric is in terms of the area, so our method with 20% crop budget yields a cropping metric of 0.64, for example.) In order to make fair comparisons, one should choose the L1 version with crop most similar to that of the method of interest on the video set of interest, and then compare other metrics: for example, to compare BCP with L1 on the *running* set, choose L1 20 (which yields similar *cropping*) and compare the *stability* and *distortion* metrics.

L1 generally performs well in terms of both the *stability* and *distortion* metrics. In fact, the L1 algorithm explicitly optimizes related criteria, namely the acceleration of the stabilized path in log-homography path, and the difference of the affine diagonals. Generally, more restrictive crop leads to less *distortion* (as smaller corrections are applied) but allows for less aggressive corrections and hence less *stability*, although these effects are usually slight except on very unstable videos like *running*. There is a certainly an L1 tradeoff between crop and stabilization strength, but restrictive crop tends to prevent L1 from achieving tripod-stabilization but not from smoothing high-frequency shake, because of large penalties on acceleration (the third derivative) compared to the first and second derivatives, and the fact that the corrections needed to achieve tripod are typically larger than those needed to smooth shake. Hence, L1 usually achieves good *stability* (recall that this metric is based on acceleration) even with limited crop budgets: for example L1 with 10% crop is competitive in *stability* even with methods that consume considerably more crop in many categories.

Admittedly, in terms of *distortion* L1 is merely comparable, and not superior, to the top-performing methods in this study. Stabilization inherently involves tradeoffs between stability, crop, and distortion; with the tuning and crop budgets used in this study, L1 shines in *stability* and *cropping* while achieving comparable *distortion* to other methods. (Furthermore, most methods in this study are already doing well in terms of distortion *i.e.* there is not much room for improvement.) In A.3, we make comparisons to [2] that show this qualitatively: neither [2]’s nor our results suffer from visible distortion (in [2]’s method, a post-processing step helps to mitigate perspective distortion, while our method handles it directly), but our method satisfies crop constraints far more accurately.

L1 has the fastest *running time* (both overall time and smoothing/warping time) of all the methods in this comparison. (Note that the total runtime of L1 depends on the method used to analyze the input motion: with inertial sensor measurements, the analysis time is negligible and the total time is the same as the smoothing/warping time, while pixel-based analysis adds additional time to the total.) PG2 and YT are the closest to L1 in runtime (and with optimized implementations could probably be as fast as L1). The goals of PG2 (geodesic

interpolation between key frames) differ from those of L1 (cinematic trajectory, crop control, etc.); YT is based on [2], upon which our method improves, and we provide detailed comparisons to [2] in section A.3.

### A.1.1 Performance - additional comparisons

In Table 1, we compare our performance with that of the methods above as well as several other alternatives (based on their self-reported runtimes). Our method is orders of magnitude faster than the 2.5-3D methods. SFM and optical flow, the bottlenecks of some 3D methods, are improving but still costly. Our method is only comparable in performance to 2D methods like Grundmann’s (which should in principle be able to run as fast as ours). Of the 2D methods, our goals of cinematic trajectories, crop control, and saliency guidance are most closely aligned with those of Grundmann [2], and less similar to the geodesic keypoint interpolation of [15] and rolling-shutter-correction/basic smoothing of [3, 11], hence our focus on qualitative comparisons to Grundmann.

Table 1: Additional performance comparisons

| Method                               | Class | Speed    |
|--------------------------------------|-------|----------|
| Ours - inertial sensor               | 2D    | 300 fps  |
| Ours - feature-based analysis        | 2D    | 120 fps  |
| Grundmann [2] (unoptimized)          | 2D    | 20 fps   |
| Geodesic Video Stabilization [15]    | 2D    | 78 fps   |
| Cell Phone Video Inertial Sensor [3] | 2D    | 1800 fps |
| Video Rectification Cellphones [11]  | 2D    | 20 fps   |
| Spatially Temporally [12]            | 2.5D  | fps      |
| Epipolar Geometry [1]                | 2.5D  | 30 fps   |
| Bundled Camera Paths [9]             | 2.5D  | 3 fps    |
| Subspace Video Stabilization [7]     | 2.5D  | 4 fps    |
| SteadyFlow (optical flow-based) [10] | 2.5D  | 0.7 fps  |
| MeshFlow [8]                         | 2.5D  | 5 fps    |
| Content-Preserving Warps [6]         | 3D    | (SFM)    |
| First-person Hyper-Lapse [5]         | 3D    | (SFM)    |

### A.2. Homography versus Affine model

One of our main contributions is direct optimization with homographies (via log-homographies) rather than affines, as used in the convex formulation of [2] and other L1 methods. Homographies can correct keystone, while affines cannot. (As discussed in the next section, [2] follow their affine solve with a ‘residual motion suppression’ step which helps clean up the keystone wobble, but also unfortunately consumes additional crop over the user-specified budget; in contrast, our method solves directly with homography, making such post-processing unnecessary.) Supplemental videos *fountain-l1-affine.mp4* and *wakatipu-l1-affine.mp4* (video credit: Gordon Laing/cameralabs) contrast our log-homography L1 method with a simpler version of our method restricted to affinities. Both examples show how affine-only stabilization results in residual keystone wobble, while our approach fully corrects the shake. To more clearly see how the underlying frame is warped via either affine or homography, see the uncropped version of the first example: *fountain-l1-affine-uncropped.mp4*. Figure 1 shows translation and keystone plots for the latter video.

### A.3. Detailed comparison to Grundmann *et al.*

Next, we compare to the method of Grundmann *et al.* [2]. [2] actually use a hybrid approach, which they call ‘Residual Motion (Wobble and Rolling Shutter) Suppression’, combining similarity transforms and homographies: similarity transforms (which have only 4 degrees of freedom) are used in the convex formulation to find the optimal path, but the optimal path is only applied every 30 frames; for intermediate frames, they decompose the optimal path into the input similarity transform and a residual, then replace the input transform with a homography. Because of the post-processing with homographies, they do not suffer from the severe residual keystone seen in the previous section. However, the post-processing step can consume a very large amount of crop over and above the fraction allowed in the optimization.

Comparisons are shown in *grundmann-gleicher4.mp4*, *grundmann-sam1.mp4*, *grundmann-lf-juggle.mp4*, and *grundmann-sany0025.mp4*. (Note that we restricted ourselves to the subset of videos in [1]’s dataset for which direct academic attribution [2, 7] was possible. Videos sourced from YouTube were excluded.) Our results are generally similar to those of [2] in terms of smoothness, but our method can more

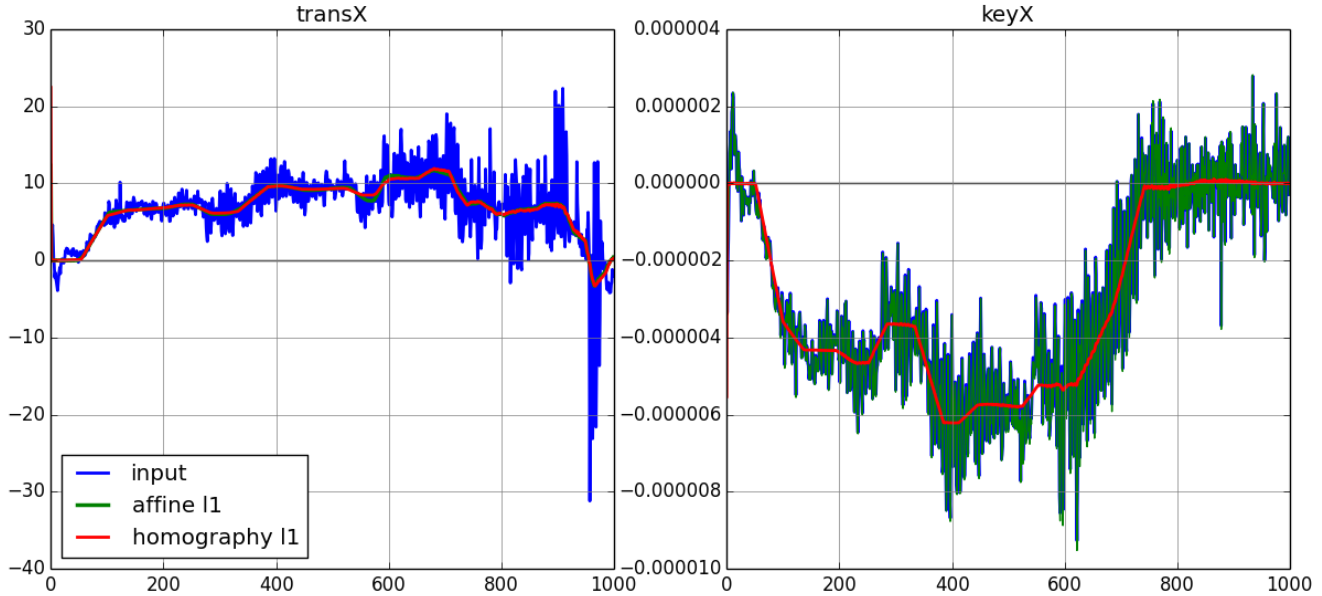

Figure 1: L1 stabilization with a log-homography model vs. affinity model. The subplots show the value over time of  $x$ -translation and  $x$ -keystone, respectively (where homographies map between consecutive frames) corresponding to video *wakatipu-l1-affine.mp4*. The homography model (red) can correct both translation and keystone resulting in smooth paths, while the affine-only model (green) smooths the translation but ignores the keystone, leaving the original shaky path (blue) only partially corrected.

rigorously satisfy crop and other constraints. This is most apparent in *grundmann-gleicher4.mp4*, where [2]’s result, which they labeled as 30% crop fraction, actually has a much smaller field-of-view (presumably due to the homography post-processing). We compare it to our results with both 30% and 40% crop fraction (which our method can strictly enforce) – [2]’s “30%” result is actually much closer to 40% crop. For the remaining three videos, [2]’s method does not seriously overconsume crop, presumably because the input videos do not have severe keystone. We find that our results are visually fairly similar to [2]’s for these less-challenging videos.

#### A.4. Ablation study

We performed an ablation study to isolate the effects of individual objective terms and constraints. This allows for quantitative comparisons, albeit in terms of our own metrics. Results are provided in table 2. The study was performed by removing objective terms and constraints from the formulation one-by-one. The videos associated with the study are *fountain-ablation-derivatives.mp4* and *fountain-ablation-innovations.mp4*.

In a related study, we set various crop budgets and window lengths/strides, and compared the results, as shown in table 3 (this was not an ablation study per se as L1 intentionally offers the client control over crop budget and window parameters, but it is similar in spirit). The corresponding videos are *fountain-crop-compare.mp4* and *fountain-l1-affine.mp4* (which shows the 30/20 frame windowed result; the 50/20 result is visually indistinguishable).

#### A.5. Additional results

**Windowing** We have included windowed-L1 results for a few of our examples (e.g. *fountain-l1-affine.mp4* and *wakatipu-l1-affine.mp4*) to show that, with sufficient lookahead, windowing has no adverse effect on stabilization quality. (Usually the lookahead need not be very large: for the two examples just mentioned, lookaheads of 2s and just 10 frames, respectively, were perfectly adequate.) One failure case that we know of is shown in *slow-pan-windowed.mp4*, where the input is an extremely slow pan, so that with too short a lookahead (5 frames or 0.25 seconds in this case), windowed-L1 can be ‘tricked’ into doing tripod-stabilization where it should not. However, with a longer lookahead (60 frames or one second in this example), windowed-L1 is very close to the global solution.

**Comparison to simple methods** Supplemental video *fountain-tripod-smooth-l1.mp4* contrasts our method with simpler approaches like tripod-mode and Gaussian smoothing, as discussed in figure 2 of the main paper (derivative plots for the video are shown in supplement 4).

**Very shaky video and the log approximation** The fact that the log approximation only holds in a neighborhood of the identity might raise concern about our method’s behavior on very shaky video. However, *wakatipu-l1-affine.mp4* (please compare the ‘input’ and ‘l1 ho-

Figure 2: Ablation study, in which we ‘turn off’ objective terms and constraints one-by-one and measure the overall objective value as well as various subobjective terms (each of which has an interpretable meaning): ‘fidelity’ is the  $\ell_2$  penalty on the corrections, measuring closeness to input, ‘1st/2nd/3rd derivatives’ are the  $\ell_1$  penalties on the derivatives of the smoothed path (zero value for each would correspond to tripod/pan/constant-acceleration, respectively) and ‘affine-diag/off-diag’ are distortion penalties as described in section 2.5 of the main paper. The crop budget is always 10% (*i.e.* we must preserve 90% of the original field-of-view), and we measure the achieved crop fraction in terms of both pixel-dimension and field-of-view. As expected, removing each derivative term (by setting the weight to zero) results in an increase in the corresponding metric relative to the reference (also, notice that in the associated video, *fountain-ablation-derivatives.mp4*, ‘minus 1st derivative’ has no tripod-stabilized segments, while the reference does). Next we consider the effects of our specific innovations relative to the method of [2]: log-homographies versus affines, field-of-view constraints, fidelity term, and additional distortion controls. With an affine-only model, the 2nd and 3rd derivatives are orders of magnitude higher than the reference owing to the uncorrected keystone; without the field-of-view constraints, the achieved field-of-view is only 82% when 90% was required; without the fidelity term, the stabilized result is further from the input trajectory; and without our distortion controls, the distortion is significantly higher. The qualitative impact of removing each term is clear in the associated video, *fountain-ablation-innovations.mp4*.

| fountain-input.mov       | reference<br>(10% crop) | minus<br>fidelity term<br>(q0=0) | minus 1st<br>derivative<br>(w1=0) | minus 2nd<br>derivative<br>(w2=0) | minus 3rd<br>derivative<br>(w3=0) | affine-only     | minus field-<br>of-view<br>constraint | minus<br>distortion<br>objective |
|--------------------------|-------------------------|----------------------------------|-----------------------------------|-----------------------------------|-----------------------------------|-----------------|---------------------------------------|----------------------------------|
| objective value          | <b>0.330436</b>         | 0.254789                         | 0.066175                          | 0.302105                          | 0.301567                          | <b>4.080111</b> | 0.229645                              | 0.291003                         |
| subobj - fidelity        | <b>0.048676</b>         | <b>0.099676</b>                  | 0.019844                          | 0.044065                          | 0.044261                          | 0.027818        | 0.087275                              | 0.054176                         |
| subobj - 1st derivative  | <b>0.231209</b>         | 0.207087                         | <b>0.450951</b>                   | 0.233449                          | 0.227362                          | 0.498161        | 0.121448                              | 0.214979                         |
| subobj - 2nd derivative  | <b>0.027362</b>         | 0.024961                         | 0.032241                          | <b>0.054488</b>                   | 0.024075                          | <b>0.239917</b> | 0.011911                              | 0.021836                         |
| subobj - 3rd derivative  | <b>0.001726</b>         | 0.001652                         | 0.001353                          | 0.001918                          | <b>0.075285</b>                   | <b>0.331150</b> | 0.000612                              | 0.123455                         |
| subobj - affine-diag     | <b>0.002949</b>         | 0.003525                         | 0.000223                          | 0.002588                          | 0.003170                          | 0.000195        | 0.000357                              | <b>0.008005</b>                  |
| subobj - affine-off-diag | <b>0.002949</b>         | 0.000269                         | 0.000033                          | 0.000283                          | 0.000270                          | 0.000251        | 0.000253                              | 0.006267                         |
| crop fraction goal       | <b>0.9</b>              | 0.9                              | 0.9                               | 0.9                               | 0.9                               | 0.9             | 0.9                                   | 0.9                              |
| crop pixel fraction      | <b>0.911111</b>         | 0.916667                         | 0.904167                          | 0.911111                          | 0.909259                          | 0.904167        | 0.863889                              | 0.912963                         |
| field of view fraction   | <b>0.900431</b>         | 0.898650                         | 0.899124                          | 0.900695                          | 0.898934                          | 0.904134        | <b>0.828236</b>                       | 0.899329                         |

Figure 3: Here we set various crop budgets (1%, 10%, 20%, 30%) (*i.e.* preserve 99%, 90%, 80%, 70% field-of-view, respectively) and window lengths/strides (30/20 frames *i.e.* 10 frame lookahead, and 50/20 frames *i.e.* 30 frame lookahead), and compared the results. The subobjectives and crop measurements are the same as those in table 2. Notice that our method is able to accurately satisfy a range of crop budgets in terms of both pixel dimension and field-of-view, with only very minor violations for the 1% budget (this is due to error in the linearization of the constraints). Also, there is a tradeoff between the objective value and the crop (e.g. the objective value is 0.14 with 30% crop compared to 0.33 for 10% crop): the larger the crop budget, the more stabilization can be applied. In this example, windowing makes very little difference to the result (the objective value is very similar to the reference), even when the lookahead is very short. This is often but not always the case, as we discuss in section A.5.

| fountain-input.mov       | reference<br>(10% crop) | 1% crop<br>budget | 20% crop<br>budget | 30% crop<br>budget | window<br>30/20<br>frames | window<br>50/20<br>frames |
|--------------------------|-------------------------|-------------------|--------------------|--------------------|---------------------------|---------------------------|
| objective value          | <b>0.330436</b>         | 6.308558          | 0.201617           | 0.142913           | 0.334300                  | 0.330472                  |
| subobj - fidelity        | <b>0.048676</b>         | 0.000300          | 0.103327           | 0.110782           | 0.067122                  | 0.049168                  |
| subobj - 1st derivative  | <b>0.231209</b>         | 0.877192          | 0.081098           | 0.024577           | 0.217833                  | 0.230664                  |
| subobj - 2nd derivative  | <b>0.027362</b>         | 0.427229          | 0.008105           | 0.002279           | 0.025752                  | 0.027338                  |
| subobj - 3rd derivative  | <b>0.001726</b>         | 0.500373          | 0.000424           | 0.000108           | 0.001619                  | 0.001728                  |
| subobj - affine-diag     | <b>0.002949</b>         | 0.000047          | 0.002327           | 0.001678           | 0.004708                  | 0.003065                  |
| subobj - affine-off-diag | <b>0.002949</b>         | 0.000006          | 0.000252           | 0.000251           | 0.000270                  | 0.000295                  |
| crop fraction goal       | <b>0.9</b>              | <b>0.99</b>       | <b>0.8</b>         | <b>0.7</b>         | 0.9                       | 0.9                       |
| crop pixel fraction      | <b>0.911111</b>         | 0.988889          | 0.829630           | 0.738889           | 0.912963                  | 0.911111                  |
| field of view fraction   | <b>0.900431</b>         | <b>0.98883</b>    | <b>0.801046</b>    | <b>0.716853</b>    | 0.900445                  | 0.900391                  |

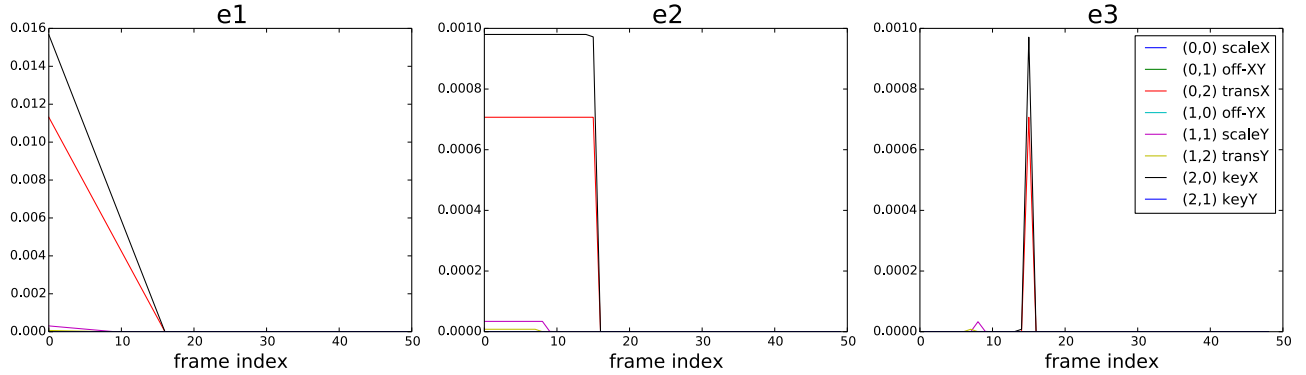

Figure 4: Derivative plots corresponding to video *fountain-tripod-smooth-l1.mp4* (discussed in figure 2 in the main text). Sparse absolute values of first ( $e^1$ ), second ( $e^2$ ), and third ( $e^3$ ) derivatives of the L1 stabilized log-homography path, per equation 4.

mography’ videos; ignore ‘l1 affine’ which is only relevant to section A.2) shows that we can successfully stabilize even very shaky video. As noted in section C, our formulation uses only transforms between consecutive input frames – which for normal frame rates should not be too large – and correction transforms. We control the correction magnitude through the  $\ell_2$  fidelity term as well as crop and distortion constraints, so for very shaky video we may not remove all the shake but we avoid making corrections severe enough to invalidate the log approximation. In practice, we have not observed any artifacts that we could attribute to the log approximation.

**Tripod and panning segments** Video *river-l1.mp4* shows the effects of sparse derivatives: the stabilized version consists of stationary and constant-velocity motions, as discussed in figure 3 of the main paper (derivative plots for the video are shown in supplement figure 5).

**Saliency results** Video *dog-l1-saliency-comparison.mp4* showcases the results of our saliency techniques (i.e. centering objectives and inclusion constraints), as discussed in figure 8 of the main paper. We chose the dog as the salient object in this video, and ran an off-the-shelf object tracker to get per-frame bounding boxes. The saliency constraints require that the bounding boxes are included in each frame of the cropped, stabilized video – notice that the trajectory changes near the end of the video to ensure that the dog is not cropped out (the slight violation is due to error associated with linearization of the constraints). The centering objective tries to keep the bounding boxes approximately centered in the frame, to the extent that the constraints and other objectives allow.

**A note on rolling-shutter correction and built-in iPhone stabilization** Our method is not designed to address rolling shutter, because there are robust existing methods to correct it [3, 11] that can and should be applied prior to stabilization. Our method is complementary to rolling shutter correction methods.

Built-in iPhone stabilization provides rolling-shutter-correction and basic Gaussian smoothing. Many of our examples were shot on modern iPhones and enjoy this stabilization, namely ‘dog’, ‘river’, and ‘slow-pan-windowed’. Our method improves these videos with precise cinematic motions, for example a jerky pan to a smooth one in ‘dog’, and drift to perfect tripod in ‘river’. Other videos came from cameras without iPhone stabilization or rolling-shutter correction (‘fountain’, all ‘grundmann’ videos, ‘wakatipu’); these demonstrate our ability to simultaneously remove high-frequency shake, partially correct rolling shutter, and create appealing cinematic trajectories.

## B. Derivative plots

The figures in this section show the absolute values of the first, second, and third derivatives of the L1 stabilized log-homography path corresponding to videos *fountain-tripod-smooth-l1.mp4* and *river-l1.mp4* (discussed in figures 2 and 3 in the main text, respectively).

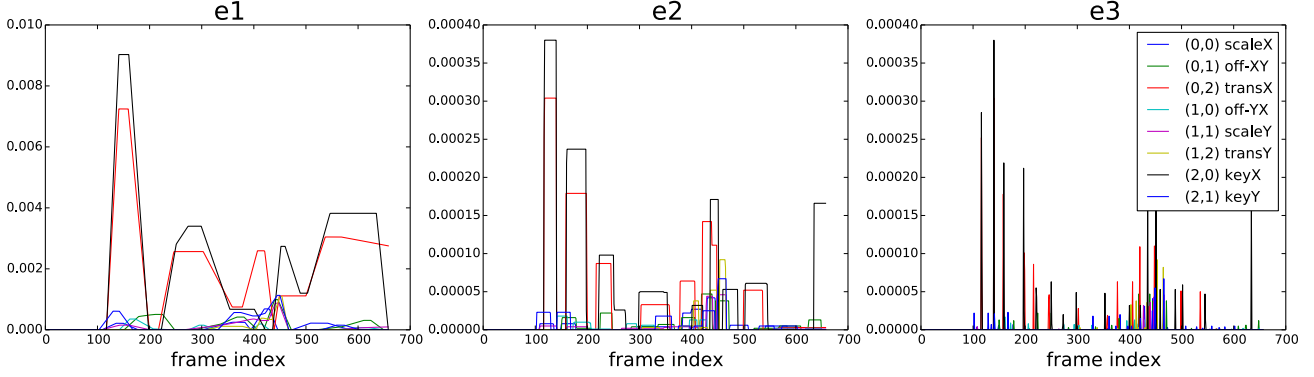

Figure 5: Derivative plots corresponding to video *river-11.mp4* (discussed in figure 3 in the main text). Sparse absolute values of first ( $e^1$ ), second ( $e^2$ ), and third ( $e^3$ ) derivatives of the L1 stabilized path (equation 4).

### C. Derivatives of corrected log-homography path

Suppose we have input homographies  $H_t$  where  $H_t$  maps frame  $t$  to  $t - 1$ , and that  $f_t = \log(H_t)$  are the corresponding log-homographies. Chaining the sequential homographies gives the homography mapping  $t$  to the identity:  $\tilde{H}_t = H_0 H_1 \dots H_t$ . Using equation 3, in terms of log-homographies this becomes approximately

$$\tilde{f}_t \approx \sum_{i=1}^t f_i. \quad (1)$$

Let  $p_t$  denote the log-correction applied to each frame; then the corrected log-path is given by:

$$\tilde{s}_t = \tilde{f}_t + p_t. \quad (2)$$

Using forward differences, the first, second, and third derivatives of the corrected log-path,  $\tilde{s}$ , are:

$$\begin{aligned} e_1(t) &= \tilde{s}_{t+1} - \tilde{s}_t \\ &= \tilde{f}_{t+1} + p_{t+1} - \tilde{f}_t - p_t \\ &= p_{t+1} + f_{t+1} - p_t \quad (\text{since } \tilde{f}_{t+1} - \tilde{f}_t = f_{t+1}) \\ \\ e_2(t) &= \tilde{s}_{t+2} - 2\tilde{s}_{t+1} + \tilde{s}_t \\ &= \tilde{f}_{t+2} + p_{t+2} - 2(\tilde{f}_{t+1} + p_{t+1}) + \tilde{f}_t + p_t \\ &= p_{t+2} + f_{t+2} - 2p_{t+1} - f_{t+1} + p_t \\ \\ e_3(t) &= \tilde{s}_{t+3} - 3\tilde{s}_{t+2} + 3\tilde{s}_{t+1} - \tilde{s}_t \\ &= \tilde{f}_{t+3} + p_{t+3} - 3(\tilde{f}_{t+2} + p_{t+2}) + 3(\tilde{f}_{t+1} + p_{t+1}) - \tilde{f}_t - p_t \\ &= p_{t+3} + f_{t+3} - 3p_{t+2} - 2f_{t+2} + 3p_{t+1} + f_{t+1} - p_t \end{aligned}$$

Since the approximation 3 only holds in a neighborhood of the identity (*i.e.* the zero matrix), equation 1 is a (possibly catastrophically) poor approximation, since addition of log-homographies accumulates error. For this reason, we avoid using  $s_t$  (which involves  $\tilde{f}_t$ ) directly in our formulation, and instead only use its derivatives which do not involve  $\tilde{f}_t$  but only sums and differences of small numbers of  $f_t$  and  $p_t$ . We can assume that the individual  $f_t$  and  $p_t$  are small, as the  $f_t$  map consecutive frames that are close in time, and the  $p_t$  are corrections to each frame that are controlled by constraints and objectives on the problem to keep them relatively close to zero.

### D. Point-delta linearization via the Jacobian

Linearization of the point-delta function is an important technical device that facilitates both the crop and saliency constraints. Consider a point-delta function  $\tilde{d} : \mathbb{R}^9 \times \mathbb{R}^2 \rightarrow \mathbb{R}^2$ ,

$$\tilde{d}(H; x) = Hx - x = \begin{bmatrix} h_0 x_0 + h_1 x_1 + h_2 \\ h_6 x_0 + h_7 x_1 + h_8 \\ h_3 x_0 + h_4 x_1 + h_5 \\ h_6 x_0 + h_7 x_1 + h_8 \end{bmatrix} - x,$$

where  $H$  is a homography and  $x \in \mathbb{R}^2$  is a point, and  $Hx$  is the homogeneous action of  $H$  on  $x$ . The gradient of  $\tilde{d}$  with respect to  $H$  (with  $x$  considered a fixed parameter) is:

$$\begin{aligned} \nabla \tilde{d}|_{H,x} &= \begin{bmatrix} \frac{x_0}{h_6 x_0 + h_7 x_1 + h_8} & \frac{x_1}{h_6 x_0 + h_7 x_1 + h_8} & \cdots & \frac{-x_0(h_0 x_0 + h_1 x_1 + h_2)}{(h_6 x_0 + h_7 x_1 + h_8)^2} & \cdots & \frac{-(h_0 x_0 + h_1 x_1 + h_2)}{(h_6 x_0 + h_7 x_1 + h_8)^2} \\ \vdots & \vdots & & & & \end{bmatrix} \\ \Rightarrow \nabla \tilde{d}|_{I,x} &= \begin{bmatrix} x_0 & x_1 & 1 & 0 & 0 & 0 & -x_0^2 & -x_0 x_1 & -x_0 \\ 0 & 0 & 0 & x_0 & x_1 & 1 & -x_0 x_1 & -x_1^2 & -x_1 \end{bmatrix} \end{aligned}$$

Now, define

$$d(h; x) = \tilde{d}(\exp(h), x) \equiv Hx - x, \quad \text{where } H = \exp(h)$$

The first order approximation at  $h = 0$  is given by:

$$d(h; x) \approx \nabla d|_{0,x} h,$$

where  $\nabla d|_{h,x}$  is the Jacobian with respect to  $h$ . By the argument in D.1, at the identity  $h = 0$ :

$$\nabla d|_{0,x} = \nabla \tilde{d}|_{I,x}.$$

Now consider a function  $D(h; c^{0:4}) : \mathbb{R}^9 \rightarrow \mathbb{R}^8$  that computes the point-delta due to  $h$  for four corners (in known, fixed positions; we consider these parameters to the function rather than independent variables). The Jacobian of  $D$  with respect to  $h$  at the identity log-homography is given by:

$$\nabla D|_{0,c^{0:4}} = \begin{bmatrix} c_0^{(0)} & c_1^{(0)} & 1 & 0 & 0 & 0 & -c_0^{(0)2} & -c_0^{(0)} c_1^{(0)} & -c_0^{(0)} \\ 0 & 0 & 0 & c_0^{(0)} & c_1^{(0)} & 1 & -c_0^{(0)} c_1^{(0)} & -c_1^{(0)2} & -c_1^{(0)} \\ \vdots & \vdots \\ c_0^{(3)} & c_1^{(3)} & 1 & 0 & 0 & 0 & -c_0^{(3)2} & -c_0^{(3)} c_1^{(3)} & -c_0^{(3)} \\ 0 & 0 & 0 & c_0^{(3)} & c_1^{(3)} & 1 & -c_0^{(3)} c_1^{(3)} & -c_1^{(3)2} & -c_1^{(3)} \end{bmatrix} \in \mathbb{R}^{8 \times 9} \quad (3)$$

We can apply the Jacobian to the corners of the video frame, in combination with the chain rule, to compute the change in quantities that depend on the mapped corner positions.

### D.1. Gradient of function of log-homography at identity

In general, given a function  $\tilde{f}(H)$  acting on homographies, consider

$$f(h) = \tilde{f}(\exp h),$$

acting on log-homographies. Then the Jacobians of  $f$  and  $\tilde{f}$  agree at the identity (though not elsewhere):

$$\begin{aligned} \nabla_h f(h) &= \nabla_h \tilde{f}(\exp(h)) \\ &= \nabla_H \tilde{f} \circ \nabla_h H \quad \text{where } H = \exp(h) \quad (\text{by the chain rule}) \\ \exp(h) &= \sum_{n=0}^{\infty} \frac{h^n}{n!} = I + h + \frac{1}{2}h^2 + \dots \Rightarrow \nabla_h \exp(h) = I + \nabla_h \left(\frac{1}{2}h^2 + \dots\right) \\ \Rightarrow \nabla_h H(0) &= I \quad (\text{note that this holds only at } h = 0) \\ \Rightarrow \nabla_h f(0) &= \nabla_H \tilde{f}(I) \end{aligned}$$

## E. Gradients of area and squared-sidlength

The area and squared-sidelengths of a transformed rectangle depend on the log-homography transform  $p$  via the transformed corner positions. If  $c(p; c_0)$  computes the new corner positions under transform  $p$  for corners originally at positions  $c_0$ , then both the area and sidelength constraints can be written:

$$A(c(p; c_{\text{wind}})) \geq A_{\min},$$

where  $A(c)$  means the area/squared-sidelength of the quadrilateral with corners  $c$ , and  $c_{\text{wind}}$  are the crop window corners. To linearize those constraints, we need to compute the gradient of  $A$  with respect to  $p$ , which we can do using the chain rule:

$$\begin{aligned}\nabla_p A &= \nabla_c A(c_0)^T \nabla_p c(p; c_0) \quad \text{by the chain rule} \\ &= \nabla_c A(c_0)^T \nabla D|_{p, c_0} \quad (\text{corner positions have same gradient as point-deltas } D) \\ \implies \nabla_p A(0; c_0) &= \nabla_c A(c_0)^T \nabla D|_{0, c_0}\end{aligned}$$

Hence the linearization of the constraint about  $p = 0$  is:

$$\nabla_p A(0; c_{\text{wind}}) \equiv \nabla_c A(c_{\text{wind}})^T \nabla D|_{0, c_{\text{wind}}} \geq A_{\min} - A(c_{\text{wind}})$$

Now we just need the gradients of the area and sidelengths with respect to the corner positions,  $\nabla_c A$ . The length of a line segment between  $(x_a, y_a)$  and  $(x_b, y_b)$  is

$$l(x_a, y_a, x_b, y_b) = (x_a - x_b)^2 + (y_a - y_b)^2.$$

and its gradient is:

$$\nabla l = \begin{bmatrix} 2(x_a - x_b) & 2(y_a - y_b) & -2(x_a - x_b) & -2(y_a - y_b) \end{bmatrix}^T.$$

Recall that the area of a triangle composed of vectors  $\vec{v}$  and  $\vec{w}$  is the magnitude of  $\frac{\vec{v} \times \vec{w}}{2}$ . In two dimensions, this is just  $\frac{(v_x w_y - w_x v_y)}{2}$ . In two dimensions, this is just  $\frac{(v_x w_y - w_x v_y)}{2}$ . Since we chose the ordering of the  $\vec{q}$ 's counter-clockwise, the counter-clockwise condition will hold for our quadrilateral when  $C$  is a small homography. Therefore, the area of a quadrilateral with “reasonably” positioned points, *i.e.* no edges crossing or large exterior angles, is:

$$A(c) = ((x_1 - x_0)(y_2 - y_1) - (x_2 - x_1)(y_1 - y_0) + (x_3 - x_2)(y_0 - y_3) - (x_0 - x_3)(y_3 - y_2))/2.$$

and its gradient is:

$$\nabla_c A = \frac{1}{2} \begin{pmatrix} y_1 - y_3 & x_3 - x_1 & y_2 - y_0 & x_0 - x_2 & y_3 - y_1 & x_1 - x_3 & y_0 - y_2 & x_2 - x_0 \end{pmatrix}^T.$$

## F. Third Order Markov property

Consider the L1 problem subject to the constraint that the solution  $p$  is fixed up to frame  $s - 1$ , which means that each  $e^i$  is also fixed up to frame  $s - i - 1$  (*i.e.*  $e^1$  up to  $s - 2$ ,  $e^2$  up to  $s - 3$ ,  $e^3$  up to  $s - 4$ ):

$$\begin{aligned}\underset{p \in \mathbb{R}^{kn}}{\text{minimize}} \quad & w_1 \|e_{s-1:n}^1\|_1 + w_2 \|e_{s-2:n}^2\|_1 + w_3 \|e_{s-3:n}^3\|_1 + \frac{1}{2} w_0 \|p_{s:n}\|_2^2 \\ & + \text{const (objective for } p_{0:s-1}, e_{0:s-2}^1, e_{0:s-3}^2, e_{0:s-4}^3) \\ \text{subject to:} \quad & p_t = \tilde{p}_t \quad 0 \leq t \leq s - 1 \\ & e_t^i = L(p_{t+i}, \dots, p_t), \quad i = 1, 2, 3, \quad \forall t \\ & \text{usual constraints on } p_t, \quad t \geq s\end{aligned}$$

(Here,  $L$  is simply shorthand for the set of affine constraints that define the  $e^i$  in terms of  $p$ .) Note that the optimal solution conditional on the fixed solution  $\tilde{p}$  up to frame  $s - 1$  really only depends on  $\tilde{p}$  in frames  $s - 3, s - 2, s - 1$ . In particular,  $e_{s-3}^3$  appears in the objective and depends on  $\tilde{p}_{s-3}$ , but that's as far back as we look. Put another way, the effect of *all* previous frames is only felt through the previous 3 frames, *i.e.* the problem is Markov of order 3.

With these observations, we can write down an equivalent problem (whose objective differs only by a constant) in terms of only frames  $s - 3$  and up:

$$\begin{aligned}\underset{p_{s-3:n}}{\text{minimize}} \quad & w_1 \|e_{s-1:n}^1\|_1 + w_2 \|e_{s-2:n}^2\|_1 + w_3 \|e_{s-3:n}^3\|_1 + \frac{1}{2} w_0 \|p_{s:n}\|_2^2 \\ \text{subject to:} \quad & p_t = \tilde{p}_t \quad s - 3 \leq t \leq s - 1 \\ & e_t^i = L(p_{t+i}, \dots, p_t), \quad i = 1, 2, 3, \quad t \geq s - 3 \\ & \text{usual constraints on } p_t, \quad t \geq s\end{aligned}$$

(Note that  $e_{s-3}^3$  links the first unknown variable  $p_s$  with  $\tilde{p}_{s-3}$ .) This reformulation tells us that if we wish to solve the full problem subject to  $p_t = \tilde{p}_t$  for all  $t \leq s - 1$ , we just ‘restart’ at frame  $s - 3$  (ignore all frames prior to  $s - 3$ ) and initialize  $p_{s-3, s-2, s-1}$  to the corresponding  $\tilde{p}$  (this is equivalent to initializing  $p_{s-3}, e_{s-3}^1, e_{s-3}^2$ , and both imply that all of  $p_{s-3, s-2, s-1}, e_{s-3, s-2}^1, e_{s-3, s-2}^2$  are constrained.)

It can be somewhat confusing whether we need 3 or 4 frames of initialization. It's actually just 3:  $\tilde{p}_{s-3, s-2, s-1}$  – which is equivalent to  $p, e^1, e^2$  at  $s - 3$ . We already know  $p$  up to frame  $s - 1$  and we're trying to find it for frame  $s$  onward, so there is no point adding the variable  $\tilde{p}_{s-4}$  since its value is already known and it contains no useful information through any derivative about frames  $s$  onward (it wouldn't hurt anything to add it, but it's unnecessary).

## G. Keystone-translation relationship via infinite homographies

Much of the following is adapted from [4]. Suppose we have camera matrices (ignoring intrinsics for now)

$$P = [I|0], \quad P' = [R|t],$$

with  $R \in \mathbb{R}^{3 \times 3}$  a 3D rotation matrix and  $t \in \mathbb{R}^3$  a translation (represented homogeneously), and a world plane  $\pi = (v, 1)$  defined by  $\pi^T X = 0$ . The homography induced by this plane (i.e the homography that transfers  $x$  in first view to  $x'$  in second view by first back-projecting  $x$  onto  $\pi$  and then projecting the resulting 3D point to  $x'$ ) is  $x' = Hx$  with  $H = R - tv^T$ . If  $v = (n, d)$ , i.e. points on the plane satisfy  $n^T X + d = 0$ , this becomes

$$H = R - tn^T/d.$$

The ‘infinite homography’ is induced by the plane at infinity, i.e. the limit as  $d \rightarrow \infty$  (world plane gets infinity far away):

$$H_\infty = \lim_{d \rightarrow \infty} H = R.$$

If the cameras have (simplified) intrinsics  $K, K'$ , respectively, of the form  $K = \begin{bmatrix} f & 0 & 0 \\ 0 & f & 0 \\ 0 & 0 & 1 \end{bmatrix}$ , then the previous becomes:

$$H = K'(R - tv^T)K^{-1}, \quad H_\infty = K'RK^{-1}.$$

Given that the infinite homographies  $H_\infty$  correspond to 3D rotations, what does that tell us about the relationship between keystone and translation? Note that if  $\mathbf{q} = q_r + q_x \mathbf{i} + q_y \mathbf{j} + q_z \mathbf{k}$  is the quaternion representation of a 3D rotation, then the corresponding rotation matrix is:

$$R = \begin{bmatrix} 1 - 2s(q_j^2 + q_k^2) & 2s(q_i q_j - q_k q_r) & 2s(q_i q_k + q_j q_r) \\ 2s(q_i q_j + q_k q_r) & 1 - 2s(q_i^2 + q_k^2) & 2s(q_j q_k - q_i q_r) \\ 2s(q_i q_k - q_j q_r) & 2s(q_j q_k + q_i q_r) & 1 - 2s(q_j^2 + q_i^2) \end{bmatrix}$$

where  $s = \|q\|^{-2}$  [13].

From this, we see that if there is no  $z$ -rotation, i.e.  $q_k = 0$ , then  $r_{0,2} = -r_{2,0}$  and  $r_{1,2} = -r_{2,1}$ . Hence, if there is no  $z$ -rotation and the intrinsics are the same for both cameras ( $f$  constant but not necessarily equal to 1), then in the infinite homography  $H_\infty = K R K^{-1}$ , we have the translation-keystone relationship

$$k = -\frac{1}{f^2} t,$$

(where  $t$  is  $x$  or  $y$  translation and  $k$  is corresponding keystone entry in  $H_\infty$ ).

If we have more general rotations with  $q_k \neq 0$ , or if the focal length is variable (i.e. the camera is zooming, for example) then the situation is more complicated, and we lose the linear relationship between translation and keystone. However, in the relatively common situation where the focal length is approximately constant, and the  $z$ -rotation is small compared to  $x$  and  $y$ , then we have an approximately linear relationship between translation and keystone.

## References

- [1] Amit Goldstein and Raanan Fattal. Video stabilization using epipolar geometry. *ACM Transactions on Graphics (TOG)*, 31(5):1–10, 2012.
- [2] Matthias Grundmann, Vivek Kwatra, and Irfan Essa. Auto-directed video stabilization with robust 11 optimal camera paths. In *CVPR 2011*, pages 225–232. IEEE, 2011.
- [3] Gustav Hanning, Nicklas Forsl w, Per-Erik Forss n, Erik Ringaby, David T rnqvist, and Jonas Callmer. Stabilizing cell phone video using inertial measurement sensors. In *2011 IEEE International Conference on Computer Vision Workshops (ICCV Workshops)*, pages 1–8. IEEE, 2011.
- [4] Richard Hartley and Andrew Zisserman. *Multiple view geometry in computer vision*. Cambridge University Press, 2003.
- [5] Johannes Kopf, Michael F Cohen, and Richard Szeliski. First-person hyper-lapse videos. *ACM Transactions on Graphics (TOG)*, 33(4):1–10, 2014.
- [6] Feng Liu, Michael Gleicher, Hailin Jin, and Aseem Agarwala. Content-preserving warps for 3d video stabilization. *ACM Transactions on Graphics (TOG)*, 28(3):1–9, 2009.
- [7] Feng Liu, Michael Gleicher, Jue Wang, Hailin Jin, and Aseem Agarwala. Subspace video stabilization. *ACM Transactions on Graphics (TOG)*, 30(1):1–10, 2011.

- [8] Shuaicheng Liu, Ping Tan, Lu Yuan, Jian Sun, and Bing Zeng. Meshflow: Minimum latency online video stabilization. In *European Conference on Computer Vision*, pages 800–815. Springer, 2016.
- [9] Shuaicheng Liu, Lu Yuan, Ping Tan, and Jian Sun. Bundled camera paths for video stabilization. *ACM Transactions on Graphics (TOG)*, 32(4):1–10, 2013.
- [10] Shuaicheng Liu, Lu Yuan, Ping Tan, and Jian Sun. Steadyflow: Spatially smooth optical flow for video stabilization. In *Proceedings of the IEEE Conference on Computer Vision and Pattern Recognition*, pages 4209–4216, 2014.
- [11] Erik Ringaby and Per-Erik Forssén. Efficient video rectification and stabilisation for cell-phones. *International journal of computer vision*, 96(3):335–352, 2012.
- [12] Yu-Shuen Wang, Feng Liu, Pu-Sheng Hsu, and Tong-Yee Lee. Spatially and temporally optimized video stabilization. *IEEE transactions on visualization and computer graphics*, 19(8):1354–1361, 2013.
- [13] Wikipedia. Quaternions and spatial rotation. [https://en.wikipedia.org/wiki/Quaternions\\_and\\_spatial\\_rotation#Quaternion-derived\\_rotation\\_matrix](https://en.wikipedia.org/wiki/Quaternions_and_spatial_rotation#Quaternion-derived_rotation_matrix), 2019.
- [14] Wikipedia. Rotation matrix. <https://en.wikipedia.org/wiki/RotationMatrix>, 2019.
- [15] Lei Zhang, Xiao-Quan Chen, Xin-Yi Kong, and Hua Huang. Geodesic video stabilization in transformation space. *IEEE Transactions on Image Processing*, 26(5):2219–2229, 2017.
